# Supplementary material for: Quantized Born Effective charges as probes for the topological phase transition in the Haldane and Kane-Mele models
Source: arXiv:2404.18329 source file (2025-06-07)
Supplement: Supplementary file 1 [file SM.pdf]

# Supplementary Information for 'Quantized Born Effective charges as probes for the topological phase transition in the Haldane and Kane-Mele models'

Paolo Fachin[1], Francesco Macheda[1], Paolo Barone[2,1], and Francesco Mauri[1]

[1]Dipartimento di Fisica, Università di Roma La Sapienza, Roma, Italy
[2]CNR-SPIN, Area della Ricerca di Tor Vergata, Via del Fosso del Cavaliere 100, I-00133 Rome, Italy

## 1 Born Effective Charges

The Born effective charges can be decomposed into two contributions, the one due to the rigid displacement of the ionic charge $Z_{\text{ion}}$ and the other accounting for the polarization of the electronic charge density induced by the lattice vibrations.

$$Z^B_{s,\alpha\beta} = Z_{\text{ion}}\delta_{\alpha\beta} + Z^*_{s,\alpha\beta} \tag{1}$$

where $\alpha\beta$ are cartesian coordinates.

In the following we focus on the tight-binding approach, realized with atomic orbitals described by $|\boldsymbol{R}, s, \gamma\rangle$, where $\boldsymbol{R}, s, \gamma$ respectively is the lattice vector, the ion and the atomic orbital. The position operator is diagonal in the basis of the tight-binding orbitals with the following eigenvalues

$$\hat{\boldsymbol{r}}\,|\boldsymbol{R}, s, \gamma\rangle = (\boldsymbol{R} + \boldsymbol{\tau}_s + \boldsymbol{u}_s)\,|\boldsymbol{R}, s, \gamma\rangle \tag{2}$$

including also the ionic displacement from equilibrium $\boldsymbol{u}_s$. In this framework the Born effective charges tensor is obtained as the sum of the nuclear charge and the contribution from the electronic charge density

$$Z^B_{s,\alpha\beta} = Z_{\text{nuc}}\delta_{\alpha\beta} + Z^{\text{el}}_{s,\alpha\beta} \tag{3}$$

where

$$eZ^{\text{el}}_{s,\beta\alpha} = -\frac{\partial^2\mathcal{E}}{\partial E_\alpha \partial u_{s,\beta}} \tag{4}$$

with $\mathcal{E}$ is the electronic energy density, $E_\alpha$ the $\alpha$ component of the electric field and $u_{s,\beta}$ the displacement from equilibrium of the $s$ ion along the direction $\beta$. According to the linear response theory eq. (3) leads to

$$Z^{\text{el}}_{s,\beta\alpha} = \frac{A}{(2\pi)^2}\int_{\text{BZ}} d^2\boldsymbol{k}\,\Omega_{k_\alpha u_{s\beta}}(\boldsymbol{k}) - \sum_n^{\text{occ}} \frac{A}{(2\pi)^2}\int_{\text{BZ}} d^2\boldsymbol{k}\,\frac{N_S}{e}\,\langle\psi_{\boldsymbol{k},n}|\,\frac{\partial^2 H}{\partial E_\alpha \partial u_{s,\beta}}\,|\psi_{\boldsymbol{k},n}\rangle \tag{5}$$

where $|\psi_{\boldsymbol{k},n}\rangle$ are the eigenstates of the Hamilotonian and $N_S$ is the spin multiplicity. Since the coupling with the electric field under the scalar potential gauge is

$$H_{\rm em} = -e \sum_{\boldsymbol{R},s',\gamma} \boldsymbol{E} \cdot (\boldsymbol{R} + \boldsymbol{\tau}_{s'} + \boldsymbol{u}_{s'}) \, |\boldsymbol{R}, s', \gamma\rangle \langle \boldsymbol{R}, s', \gamma| \tag{6}$$

the mixed derivative of the Hamiltonian with respect to the electric field and the ionic displacement reads

$$\frac{\partial^2 H_{\rm em}}{\partial E_\alpha \partial u_{s,\beta}} = -\, e \frac{\partial^2}{\partial E_\alpha \partial u_{s,\beta}} \sum_{\boldsymbol{R},s',\gamma} \boldsymbol{E} \cdot (\boldsymbol{R} + \boldsymbol{\tau}_s + \boldsymbol{u}_s) \, |\boldsymbol{R}, s', \gamma\rangle \langle \boldsymbol{R}, s', \gamma| \tag{7}$$

$$= -e\delta_{\alpha\beta} \sum_{\boldsymbol{R},\gamma} |\boldsymbol{R}, s, \gamma\rangle \langle \boldsymbol{R}, s, \gamma| \tag{8}$$

Thus, the second contribution to the electronic part of the effective charges is equal to the electronic charge density $\rho_s$ on the $s$ ionic site

$$-\sum_n^{\rm occ} \frac{A}{(2\pi)^2} \int_{\rm BZ} d^2\boldsymbol{k} \frac{N_S}{|e|} \langle \psi_{\boldsymbol{k},n}| \frac{\partial^2 H}{\partial E_\alpha \partial u_{s,\beta}} |\psi_{\boldsymbol{k},n}\rangle = \rho_s \delta_{\alpha\beta} \tag{9}$$

It follow that

$$Z^{\rm el}_{s,\beta\alpha} = \frac{A}{(2\pi)^2} \int_{\rm BZ} d^2\boldsymbol{k} \Omega_{k_\alpha u_{s\beta}}(\boldsymbol{k}) + \rho_s \delta_{\alpha\beta} \tag{10}$$

and

$$Z^B_{s,\beta\alpha} = Z^{\rm el}_{s,\beta\alpha} + Z_{\rm nuc} = \frac{A}{(2\pi)^2} \int_{\rm BZ} d^2\boldsymbol{k} \Omega_{k_\alpha u_{s\beta}}(\boldsymbol{k}) + (\rho_s + Z_{\rm nuc}) \, \delta_{\alpha\beta} \tag{11}$$

In conclusion, the contribution to the Born effective charges that accounts for the non trivial arrangement of the electronic charge density induced by the lattice vibration is

$$Z^*_{s,\beta\alpha} = \frac{A}{(2\pi)^2} \int_{\rm BZ} d^2\boldsymbol{k} \Omega_{k_\alpha u_{s\beta}}(\boldsymbol{k}) \tag{12}$$

while the ionic contribution is

$$Z_{\rm ion} = Z_{\rm nuc} + \rho_s \tag{13}$$

We remark that in a tight-binding approach the relation between $Z^{\rm el}_{s,\alpha\beta}$ and $Z^*_{s,\alpha\beta}$ depends on the choice of the eigenvalues of the position operator, whereas in an *ab intio* framework the rigid ion contribution correspond to the ionic charge in a pseudopotential calculation, while the electronic contribution contains only the effect of the change in the electronic charge density due to the lattice vibration [1]–[3].

The Haldane model is spinless, so taking $N_S = 1$ and $Z_{\rm nuc} = \frac{1}{2}$ the Mulliken charges plotted in Figure 1 does not have any dependence on the topological state of the system. Moreover, varying almost linearly from $-0.08$ to $0.08$ in the topological trivial state they are small in comparison with the other contribution, while in the non trivial phase they further reduce the Born effecting charges to values closer to 0. In the Kane-Mele model, by virtue of the presence of the spin, the results are analogous with $N_S = 2$ and $Z_{\rm nuc} = 1$. In conclusion, in this work we focus on the contribution to the effective charges arising from the electronic density changes induced by the lattice vibrations, neglecting the trivial term of the Mulliken charges.

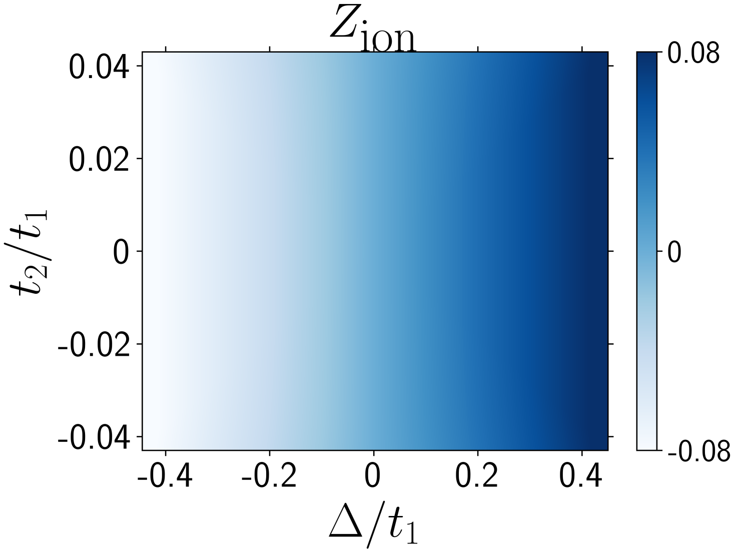


**Figure 1:** $Z_{\rm ion}$ on the ion with $l_s = 1$ for the Haldane model in the plane $(\Delta/t_1, t_2/t_1)$ for $t_1 = 3.4$ eV in the same range of parameters of Figure 1 of the main text. There is no dependence on the topological state of the system since the Mulliken charges correspond trivially the charge on each ion.

## 2 Electron-phonon coupling as a gauge field in low energy Hamiltonians

First, we show with the same formalism of the main text that, if the effective Dirac fermion Hamiltonian is spinless and obtained from a tight-binding model deriving from two orbitals on different ions, the electron-phonon coupling deriving from the variation of the hopping due to the change in the bond length enters as a gauge field. Later, we generalize the result to any tight-binding model accounting for sublattice degrees of freedom, that describes a crystalline system undergoing topological phase transition.

In a tight-binding framework the dominant contribution of the electron-phonon interaction comes from the variation of the nearest-neighbour hopping due to the ion displacement from equilibrium position, as reported in eq. (6) of the main text

$$\delta H_{\text{e-ph}} = -t_1 \xi \sum_{\langle ij \rangle} \boldsymbol{b}_{ij} \cdot (\delta \boldsymbol{u}_j - \delta \boldsymbol{u}_i)\, c_i^\dagger c_j. \tag{14}$$

In the basis of the Bloch functions obtained from the orbitals $|\boldsymbol{R}, s\rangle$ localized on the $s$ ion of the cell identified by the lattice vector $\boldsymbol{R}$

$$|\boldsymbol{k}, s\rangle = \frac{1}{\sqrt{N}} \sum_{\boldsymbol{R}} e^{i\boldsymbol{k}\cdot\boldsymbol{r}} \,|\boldsymbol{R}, s\rangle\,, \tag{15}$$

the $\boldsymbol{q}=0$ electron-phonon matrix element, due to nearest neighbours for simplicity, reads

$$\begin{aligned}
\langle \boldsymbol{k}s|\, \delta H_{\text{e-ph}}\, |\boldsymbol{k}r\rangle &= -t_1\xi \sum_j \boldsymbol{C}_j^1 e^{i\boldsymbol{k}\cdot\boldsymbol{C}_j^1} \cdot (\delta\boldsymbol{u}_s - \delta\boldsymbol{u}_r) \\
&= -it_1\xi \sum_j \frac{\partial e^{i\boldsymbol{k}\cdot\boldsymbol{C}_j^1}}{\partial\boldsymbol{k}} \cdot (\delta\boldsymbol{u}_s - \delta\boldsymbol{u}_r) \\
&= -it_1\xi \frac{\partial\left(\sum_j e^{i\boldsymbol{k}\cdot\boldsymbol{C}_j^1}\right)}{\partial\boldsymbol{k}} \cdot (\delta\boldsymbol{u}_s - \delta\boldsymbol{u}_r) \\
&= -i\xi \frac{\partial f(\boldsymbol{k})}{\partial\boldsymbol{k}} \cdot (\delta\boldsymbol{u}_s - \delta\boldsymbol{u}_r)\,,
\end{aligned} \tag{16}$$

where $\boldsymbol{C}_j^1$ are the first nearest neighbours connecting atom $s$ to atom $r$ and $f(\boldsymbol{k}) = t_1 \sum_j e^{i\boldsymbol{k}\cdot\boldsymbol{C}_j^1}$.

A gap closure associated with a topological phase transition occurs at $\boldsymbol{k}_0$, described by an effective two band model expressed in terms of $\boldsymbol{p}=\boldsymbol{k}-\boldsymbol{k}_0$, in a non orthogonal basis formed by $\{p_1,p_2\}$, obtained from linear combinations of $p_x, p_y$. For simplicity, we now consider the case where $p_1=p_x$, $\frac{\partial}{\partial p_x}=\frac{\partial}{\partial k_x}$ and $p_2=p_y$, $\frac{\partial}{\partial p_y}=\frac{\partial}{\partial k_y}$; the generalization to non orthogonal coordinates systems is trivial. Suppose that the effective model is obtained as the linear expansion of a tight-binding model built from two orbitals of different ions, that for simplicity includes only the nearest neighbour contribution. Defining the real constants $v_x = \left.\frac{\partial f(\boldsymbol{k})}{\partial k_x}\right|_{\boldsymbol{k}=\boldsymbol{k_0}}$ and $v_y = i\left.\frac{\partial f(\boldsymbol{k})}{\partial k_y}\right|_{\boldsymbol{k}=\boldsymbol{k_0}}$ the electronic Hamiltonian reads

$$H_0 = E_0\sigma_0 + v_x p_x \sigma_x^{\mathrm{P}} + v_y p_y \sigma_y^{\mathrm{P}} + m\sigma_z^{\mathrm{P}}\,, \tag{17}$$

where the Pauli matrices are defined in the pseudospin space. An analogous expansion of the electron-phonon matrix element to the leading order leads to:

$$\langle \boldsymbol{k}s|\, \delta H_{\text{e-ph}}\, |\boldsymbol{k}r\rangle = -\, i\xi v_x\left(\delta u_{s,x} - \delta u_{r,x}\right) - \xi v_y\left(\delta u_{s,y} - \delta u_{r,y}\right). \tag{18}$$

Since the Hamiltonian matrix is hermitian the electron-phonon can be expressed in terms of the Pauli matrices, defined in pseudospin space, as

$$\delta H_{\text{e-ph}} = -\,\xi v_y\left(\delta u_{s,y} - \delta u_{r,y}\right)\sigma_x^{\mathrm{P}} + \xi v_x\left(\delta u_{s,x} - \delta u_{r,x}\right)\sigma_y^{\mathrm{P}} \tag{19}$$

$\delta H_{\text{e-ph}}$ is invariant under the exchange of the indexes $s$ and $r$, since this implies a change in the sign of the nearest neighbour distance $\boldsymbol{C}_j^1$.

In conclusion, it follows that the electron-phonon coupling arising from the variation of the bond length enters as a gauge field in the low energy Hamiltonian

$$\begin{aligned}
H &= H_0 + \delta H_{\text{e-ph}} \\
&= E_0\sigma_0 + v_x(p_x + \xi\mathcal{B}_x)\sigma_x + v_y(p_y + \xi\mathcal{B}_y)\sigma_y + m\sigma_z,
\end{aligned} \tag{20}$$

where

$$\boldsymbol{\mathcal{A}}_s = -\delta u_{s,y}\hat{p_x} + \delta u_{s,x}\hat{p_y}, \quad \boldsymbol{\mathcal{B}} = \boldsymbol{\mathcal{A}}_s - \boldsymbol{\mathcal{A}}_r. \tag{21}$$

The above derivation is extended in a straightforward manner to higher order tight-binding hopping terms.

## Generalization to any tight-binding model

The result can be generalized to any topological phase transition in a crystal admitting a tight-binding description of its energy bands, starting from the basis set of the space accounting for sublattice degrees of freedom. Our derivation neglects couplings between the spin degrees of freedom and the real-space angular dependence of the electron-phonon coupling, since we assume that the electron-phonon coupling is generated only by longitudinal variations of the bond length between different site. Though, this assumption does not invalidate our analysis, since the terms that we restrict to analyze will always be present, whatever their magnitude may be.

In a generic crystalline system, we consider an electronic tight-binding Hamiltonian on a basis of $m$ ions labelled as $\{s_{j,l}\}_{j=1,..,m;l=1,..,n_j}$ with $n_j$ number of orbitals for the ion $j$, described by $|\boldsymbol{R}, s_{j,l}\rangle$ on the cell identified by the lattice vector $\boldsymbol{R}$. In the basis of the Bloch functions

$$|\boldsymbol{k}, s_{j,l}\rangle = \frac{1}{\sqrt{N}} \sum_{\boldsymbol{R}} e^{i\boldsymbol{k}\cdot\boldsymbol{r}} |\boldsymbol{R}, s_{j,l}\rangle \tag{22}$$

the $M \times M$ Hamiltonian reads

$$H_0(\boldsymbol{k}) = \begin{pmatrix} f_{s_{1,1},s_{1,1}}(\boldsymbol{k}) & f_{s_{1,1},s_{1,2}}(\boldsymbol{k}) & \dots & f_{s_{1,1},s_{2,1}}(\boldsymbol{k}) & \dots \\ f^*_{s_{1,1},s_{1,2}}(\boldsymbol{k}) & f_{s_{1,2},s_{1,2}}(\boldsymbol{k}) & \dots & & \\ \cdot & & & & \\ \cdot & & & & \\ \cdot & & & & \\ f^*_{s_{1,1},s_{2,1}}(\boldsymbol{k}) & \dots & & & \end{pmatrix} \tag{23}$$

where the $f_{s_{j,l},s_{j',m}}(\boldsymbol{k}) = \langle \boldsymbol{k}, s_{j,l}| H_0 |\boldsymbol{k}, s_{j',m}\rangle$.

Among the M bands we focus on the two bands involved in the gap closure associated with the topological phase transition occurring at the point $\boldsymbol{k}_0$. The physical properties associated with such transition are described by an effective model, that can be obtained in general from the Löwdin partitioning method [4], [5]

$$H_{\text{eff}} = \begin{pmatrix} \tilde{\Delta}_1(\{f_{s_{j,l}s_{j',m}}(\boldsymbol{k})\})) & F(\{f_{s_{j,l}s_{j',m}}(\boldsymbol{k})\})) \\ F^*(\{f_{s_{j,l}s_{j',m}}(\boldsymbol{k})\})) & \tilde{\Delta}_2(\{f_{s_{j,l}s_{j',m}}(\boldsymbol{k})\})) \end{pmatrix} \tag{24}$$

where $\{f_{s_{j,l}s_{j',m}}(\boldsymbol{k})\}$ indicates the entire set of the hopping terms of the complete Hamiltonian and $F(\{f_{s_{j,l}}(\boldsymbol{k})\}))|_{\boldsymbol{k}_0} = 0$. In the most general formulation, the effective Hamiltonian admits an expansion as a massive Dirac fermion Hamiltonian around the gap closing point in terms of the variable $\boldsymbol{p} = \boldsymbol{k} - \boldsymbol{k_0}$. As above, we consider an orthogonal cartesian basis where $p_x$, $\frac{\partial}{\partial p_x} = \frac{\partial}{\partial k_x}$ and $p_y$, $\frac{\partial}{\partial p_y} = \frac{\partial}{\partial k_y}$. The Hamiltonian takes the form

$$H = E_0\sigma_0 + v_x p_x \sigma_x + v_y p_y \sigma_y + m\sigma_z, \tag{25}$$

$$v_x = \sum_{j,j'=1}^{M} \sum_{l=1}^{n_j} \sum_{m=1}^{n_{j'}} \frac{\partial F}{\partial f_{s_{j,l}s_{j',m}}} \frac{\partial f_{s_{j,l}s_{j',m}}(\boldsymbol{k})}{\partial k_x}\Big|_{\boldsymbol{k}_0}, \tag{26}$$

$$v_y = \sum_{j,j'=1}^{M} \sum_{l=1}^{n_j} \sum_{m=1}^{n_{j'}} \frac{\partial F}{\partial f_{s_{j,l}s_{j',m}}} \frac{\partial f_{s_{j,l}s_{j',m}}(\boldsymbol{k})}{\partial k_y}\Big|_{\boldsymbol{k}_0}. \tag{27}$$

We introduce the electron-phonon coupling as the variation of the hopping term due to the change in the distance between the ions as in eq.(6) of the main text, disregarding angular dependencies.

According to Supplementary eq. (16), the electron-phonon coupling enters in each matrix element of Supplementary eq.(23) as

$$f_{s_{j,l}s_{j',m}}(\boldsymbol{k}) \to f_{s_{j,l}s_{j',m}}(\boldsymbol{k}) - i\xi_{jj'}\frac{\partial f_{s_{j,l}s_{j',m}}(\boldsymbol{k})}{\partial \boldsymbol{k}}\Big|_{\boldsymbol{k}_0} \cdot \left(\delta\boldsymbol{u}_{s_j} - \delta\boldsymbol{u}_{s_{j'}}\right), \tag{28}$$

with $\xi_{jj'} = \xi_{j'j}$ electron-phonon coupling strength between ions $j$ and $y$. With such substitution

$$F(\{f_{s_{j,l}}(\boldsymbol{k}) - i\xi_{jj'}\frac{\partial f_{s_{j,l}s_{j',m}}(\boldsymbol{k})}{\partial \boldsymbol{k}} \cdot \left(\delta\boldsymbol{u}_{s_j} - \delta\boldsymbol{u}_{s_{j'}}\right)\}))|_{\boldsymbol{k}_0} \neq 0. \tag{29}$$

the series expansion of $F$ around $\boldsymbol{k}_0$ admits a zero order term

$$F^{(0)} = -i\sum_{j,j'=1}^{M}\sum_{l=1}^{n_j}\sum_{m=1}^{n_{j'}}\xi_{jj'}\frac{\partial F}{\partial f_{s_{j,l}s_{j',m}}}\frac{\partial f_{s_{j,l}s_{j',m}}(\boldsymbol{k})}{\partial \boldsymbol{k}}\Big|_{\boldsymbol{k}_0} \cdot \left(\delta\boldsymbol{u}_{s_j} - \delta\boldsymbol{u}_{s_{j'}}\right). \tag{30}$$

Performing the computation with such substitution, one ends up with the same results as doing the following substitution in Eq. (25)

$$v_\alpha p_\alpha \to v_\alpha p_\alpha - i\sum_{j=1}^{M}\tilde{v}_{s_j,\alpha}\delta u_{s_j,\alpha}, \tag{31}$$

$$\tilde{\boldsymbol{v}}_{s_j} = \sum_{j'=1}^{M}\sum_{l=1}^{n_j}\sum_{m=1}^{n_{j'}}\xi_{jj'}\frac{\partial F}{\partial f_{s_{j,l}s_{j',m}}}\frac{\partial f_{s_{j,l}s_{j',m}}(\boldsymbol{k})}{\partial \boldsymbol{k}}, \tag{32}$$

where $f_{s_{j,l}s_{j',m}} = f^*_{s_{j',m}s_{j,l}}$.

In conclusion, for a crystalline system that can be described by a tight-binding model, starting from the basis set accounting for the sublattice degrees of freedom, undergoing a topological phase transition associated to a gap closure, the electron-phonon coupling has a component that enters a gauge field in the massive Dirac fermion effective Hamiltonian as in (31).

# 3 Tight-binding solution of the Haldane and Kane-Mele model

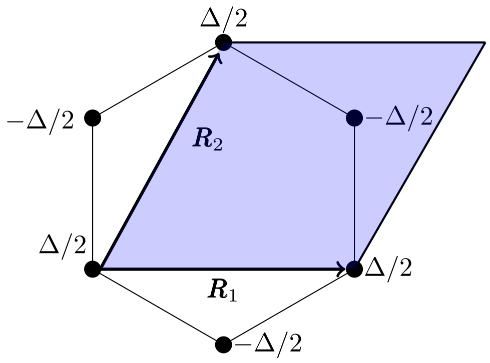


**Figure 2:** Gapped graphene structure, with the direct lattice vectors indicated as $\boldsymbol{R}_1$ and $\boldsymbol{R}_2$. The atomic sites are identified by black circles and labelled with the on-site energy. The blue region is the unit cell generated by the direct lattice vectors.

The Haldane model is defined on an hexagonal lattice, as in Fig. 2, generated by the lattice vectors

$$\boldsymbol{R_1} = (1,0)a, \quad \boldsymbol{R_2} = (\frac{1}{2}, \frac{\sqrt{3}}{2})a, \tag{33}$$

with a two atom basis

$$\boldsymbol{\tau_1} = (0,0)\,a, \qquad \boldsymbol{\tau_2} = \left(0, \frac{1}{\sqrt{3}}\right)a, \tag{34}$$

where $a = 2.46\,\text{Å}$ is the lattice parameter. The first nearest neighbours are defined, following the notation in Ref. [6], as

$$\boldsymbol{C}_1^1 = \left(0, \frac{1}{\sqrt{3}}\right)a, \qquad \boldsymbol{C}_1^2 = \left(-\frac{1}{2}, -\frac{\sqrt{3}}{2}\right)a, \qquad \boldsymbol{C}_1^3 = \left(\frac{1}{2}, -\frac{\sqrt{3}}{2}\right)a, \tag{35}$$

and the second nearest neighbours are defined according to Ref. [7] as

$$\boldsymbol{C}_2^1 = -\boldsymbol{R}_1, \qquad \boldsymbol{C}_2^2 = \boldsymbol{R}_2, \qquad \boldsymbol{C}_2^3 = \boldsymbol{R}_1 - \boldsymbol{R}_2, \tag{36}$$

$$\boldsymbol{C}_2^4 = \boldsymbol{R}_1, \qquad \boldsymbol{C}_2^5 = -\boldsymbol{R}_2, \qquad \boldsymbol{C}_2^6 = \boldsymbol{R}_2 - \boldsymbol{R}_1. \tag{37}$$

The reciprocal space Hamiltonian of the Haldane model $H_{\boldsymbol{k}}$ is a $2 \times 2$ matrix

$$H_{\boldsymbol{k}} = \begin{pmatrix} \frac{\Delta}{2} - g(\boldsymbol{k}) & f(\boldsymbol{k}) \\ f^*(\boldsymbol{k}) & -\frac{\Delta}{2} + g(\boldsymbol{k}) \end{pmatrix}, \tag{38}$$

where $\Delta/2$ is the onsite energy,

$$f(\boldsymbol{k}) = t_1 \sum_j e^{i\boldsymbol{k}\cdot\boldsymbol{C}_j^1} \tag{39}$$

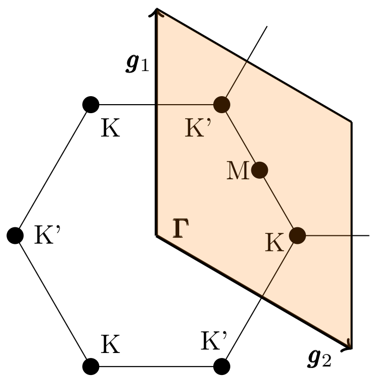


**Figure 3:** Graphene reciprocal lattice space. The first Brilluoin zone, generated by the reciprocal lattice vectors $\boldsymbol{g}_1$ and $\boldsymbol{g}_2$ with the origin in the $\Gamma$ point, is coloured in light orange. The symmetry points K, K' and M are identified by black circles. The black hexagon corresponds to the reciprocal space unit cell.

and

$$g(\boldsymbol{k}) = 2t_2 \sum_{l=1}^{3} \sin(\boldsymbol{k} \cdot \boldsymbol{C}_j^2). \tag{40}$$

$t_1$ and $t_2$ the first and the imaginary second nearest neighbour hopping. Since the set of the Pauli matrices and the identity in the two dimensional space form a complete basis of the $2 \times 2$ matrices, $H_{\boldsymbol{k}}$ can be decomposed on this basis. Namely,

$$f(\boldsymbol{k}) = t_1 \sum_j e^{i\boldsymbol{k}\cdot\boldsymbol{b}_j} = t_1 \sum_j \left(\cos\left(i\boldsymbol{k}\cdot\boldsymbol{b}_j\right) + i\sin\left(i\boldsymbol{k}\cdot\boldsymbol{b}_j\right)\right) = f_1(\boldsymbol{k}) + if_2(\boldsymbol{k}), \tag{41}$$

from which it follows that

$$H_{\boldsymbol{k}} = \begin{pmatrix} \frac{\Delta}{2} - g(\boldsymbol{k}) & f_1(\boldsymbol{k}) + if_2(\boldsymbol{k}) \\ f_1(\boldsymbol{k}) - if_2(\boldsymbol{k}) & -\frac{\Delta}{2} + g(\boldsymbol{k}) \end{pmatrix}. \tag{42}$$

Finally

$$H_{\boldsymbol{k}} = \left(f_1(\boldsymbol{k}), -f_2(\boldsymbol{k}), \frac{\Delta}{2} - g(\boldsymbol{k})\right) \cdot \boldsymbol{\sigma}^{\mathrm{P}} \quad \boldsymbol{\sigma}^{\mathrm{P}} = (\sigma_x, \sigma_y, \sigma_z)\,. \tag{43}$$

$\boldsymbol{\sigma}^{\mathrm{P}}$ is the vector of Pauli matrices in the pseudospin space. The $2 \times 2$ matrix can be solved exactly analytically with eigenvalues

$$E_{c,v} = \frac{1}{2}\sqrt{(\Delta - 2g(\boldsymbol{k}))^2 + 4|f(\boldsymbol{k})|^2}. \tag{44}$$

$c, v$ indicate conduction and valence band respectively, and eigenvectors

$$u_{\boldsymbol{k}}^c = \frac{1}{\sqrt{2}} \begin{pmatrix} \sqrt{1 + \frac{(\Delta - 2g(\boldsymbol{k}))}{2E}} \\ \frac{f^*(\boldsymbol{k})}{|f(\boldsymbol{k})|}\sqrt{1 - \frac{(\Delta - 2g(\boldsymbol{k}))}{2E}} \end{pmatrix}, \tag{45}$$

$$u_{\boldsymbol{k}}^v = \frac{1}{\sqrt{2}} \begin{pmatrix} \sqrt{1 - \frac{(\Delta - 2g(\boldsymbol{k}))}{2E}} \\ -\frac{f^*(\boldsymbol{k})}{|f(\boldsymbol{k})|}\sqrt{1 + \frac{(\Delta - 2g(\boldsymbol{k}))}{2E}} \end{pmatrix}. \tag{46}$$

The exact eigenvectors and eigenvalues are used to numerically integrated the Berry curvatures in the entire Brillouin zone on a uniform grid.
The Kane-Mele model has a $4\times4$ reciprocal space Hamiltonian that has been diagonalised numerically to compute the Berry curvatures. In order to achieve a faster convergence a telescopic grid, centred around the K and K' points, has been employed ensuring convergence with a much lower number of points with respect to a uniform one. As a matter of fact the use of the telescopic grid allows to reduce by more than two orders of magnitude the number of points needed to achieve convergence. The use of the such kind of grid is due to the fact the Berry curvatures assumes non vanishing values only in neighbouring region of such reciprocal space points, as shown in the next section. The telescopic grid is generated according to the procedure described in the Appendix B of [8] with the following parameters $\mathcal{N} = 18$, $l = 5$, $L = 11$, $p = 4$ and it is plotted in Fig. 4, highlighting the elevated density around the K and K' points.

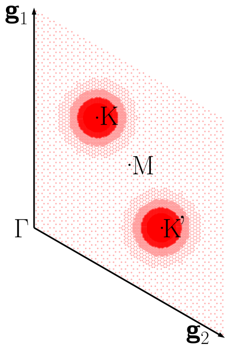


**Figure 4:** Reciprocal space telescopic grid used to numerically solve the Kane-Mele model. The poins are concentrated around the K and K'.

# 4 Conic approximation for the Berry curvatures

The low energy approximation of the three Berry curvatures $\Omega_{k_xk_y}(\mathbf{k})$,$\Omega_{k_\alpha u_{s\beta}}(\mathbf{k})$, $\Omega_{u_{s\alpha}u_{r\beta}}(\mathbf{k})$, carried out to analytically confirm the tight-binding numerical results, are justified by the fact that if the gap is sufficiently small they are localised around the K and K' points. This is shown for the Haldane model in Fig.s 5, 6 and 7. $\Omega_{u_{s\alpha}u_{r\beta}}(\mathbf{k})$ is the curvature that witness the largest variations from the low energy approximation in the region of parameter space explored in this work. For $\Delta/t_1 = 0.03$ and $0.015 < t_2/t_1 < 0.06$, all the Berry curvatures are non vanishing only in a limited region around the K and K' points. For a larger gap corresponding to $t_2/t_1 = 0.15$, the source of the curvature is less localized, covering a larger region of the Brillouin zone. Thus the error brought by the low energy approximation increases. Since the energy gap of the Haldane model is given by $|\Delta - 6\sqrt{3}t_2|$, for $\Delta/t_1 \sim 0$ and $t_2/t_1 \sim 0.1$, the gap becomes comparable with $t_1$ and the low energy approximation looses validity.

We now prove more in detail the formula obtained in the main text. Consider the Chern number as defined in eq. (2) of the main text, that in the two band system that is the Haldane model reduces to

$$C = \frac{1}{2\pi}\int_{\mathrm{BZ}} d^2\boldsymbol{k}\Omega_{k_xk_y}(\mathbf{k}).$$

Because of the localisation of the curvature around the K and K' points, a low energy expansion of the Hamiltonian around the K and K' points is justified in terms of variables $\boldsymbol{K}+\boldsymbol{p}$ and $\boldsymbol{K'}-\boldsymbol{p}$,

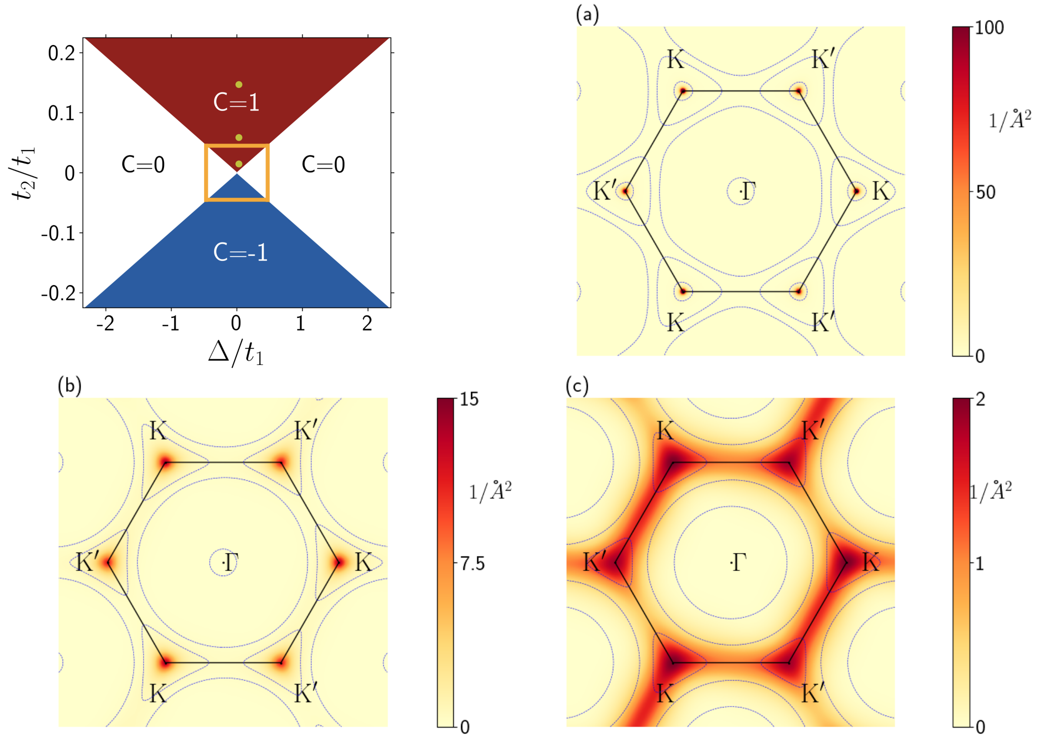


**Figure 5:** (Top left) Phase diagram of the Haldane model. The region explored in the main text is the one inside the orange square. The points indicate the values of the parameters used for the plots (a)-(b)-(b). Heat maps of $\Omega_{k_xk_y}(\mathbf{k})$ displayed on the graphene reciprocal lattice in the nontrivial phase, with $\Delta/t = 0.03$ and (a) $t_2/t = 0.015$, (b) $t_2/t = 0.06$, (c) $t_2/t = 0.15$. The three points are colored in yellow in the phase diagram. The superimposed blue dashed line are isoenergetic curves.

thus the sum over all the Brillouin zone is thus replaced by the sum of two integrals limited to neighbouring regions of the two cones $\int_{\text{BZ}} d^2\boldsymbol{k} \to \sum_{\eta=\pm1}\int_{D_\eta} d^2\boldsymbol{p}$ where $D_\eta$ is the region around each valley. Therefore:

$$C = \frac{1}{2\pi}\int_{\text{BZ}} d^2\boldsymbol{k}\Omega_{k_xk_y}(\mathbf{k}) = \frac{1}{2\pi}\sum_{\eta=\pm1}\int_{D_\eta} d^2\boldsymbol{p}\Omega_{p_xp_y}(\mathbf{p}). \tag{47}$$

The integral of the Berry curvature around each fo the two valleys is equal to a fractional Chern number [1]

$$\int_{D_\eta} d^2\boldsymbol{p}\Omega_{p_xp_y}(\mathbf{p}) = C_\eta, \tag{48}$$

where the values for $C_\eta$ in dependence of the topological phases are given in the main text. We thus arrive to

$$C = \sum_{\eta=\pm1}(\eta)^0 C_\eta. \tag{49}$$

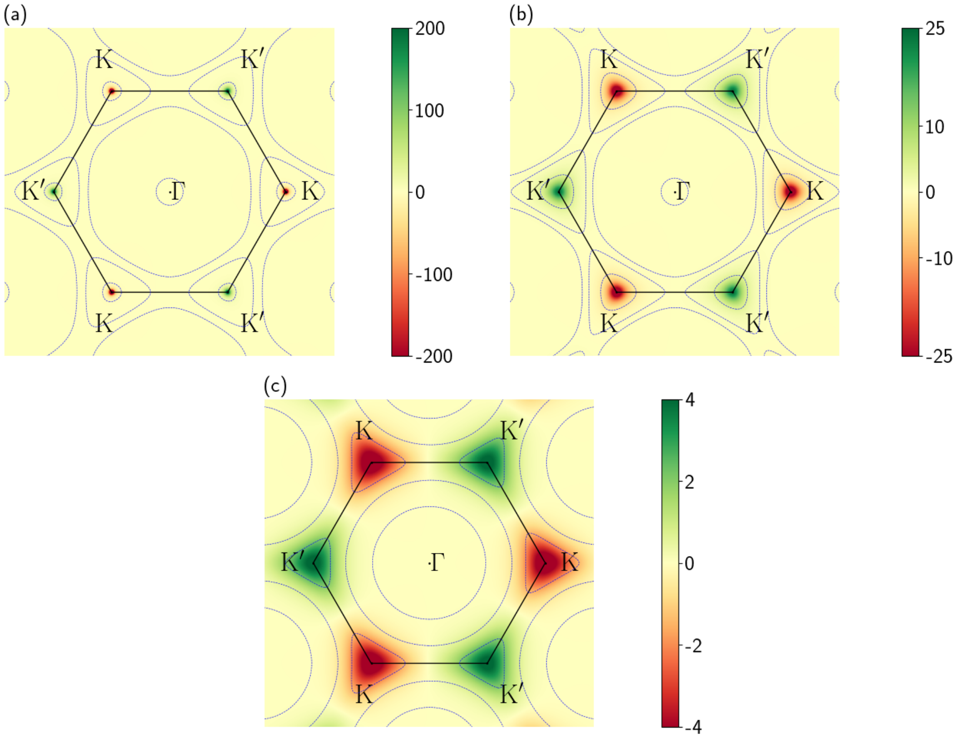


**Figure 6:** Same of Fig. 5, but for $\Omega_{k_x u_{sx}}(\mathbf{k}) + \Omega_{k_y u_{sy}}(\mathbf{k})$, with $l_s = 1$.

Thanks to the low energy expansion derivatives with respect to phonon perturbation can be recasted in terms of derivatives with respect to the crystalline quasi-momentum, as described in the main text. Consider the Born Effective charges, defined as

$$Z^*_{s,\beta\alpha} = \frac{A}{(2\pi)^2} \int_{\mathrm{BZ}} d^2\boldsymbol{k} \Omega_{k_\alpha u_{s\beta}}(\mathbf{k}). \tag{50}$$

In the Haldane model the expression reads as

$$Z^*_{s,\beta\alpha} = \frac{A}{(2\pi)^2} \int_{\mathrm{BZ}} d^2\boldsymbol{k} \Omega_{k_\alpha u_{s\beta}}(\mathbf{k}) = -\frac{A}{(2\pi)^2} \int_{\mathrm{BZ}} d^2\boldsymbol{k} \mathrm{Im} \frac{\langle \upsilon_{v\boldsymbol{k}} | \partial_{k_\alpha} H_{\boldsymbol{k}} | \upsilon_{c\boldsymbol{k}} \rangle \langle \upsilon_{c\boldsymbol{k}} | \partial_{u_{s\beta}} H_{\boldsymbol{k}} | \upsilon_{v\boldsymbol{k}} \rangle}{(\epsilon_{v\boldsymbol{k}} - \epsilon_{c\boldsymbol{k}})^2}, \tag{51}$$

and in the conic approximation reduces to

$$Z^*_{s,\beta\alpha} = \frac{A}{(2\pi)^2} \sum_{\eta=\pm1} \eta \int_{D_\eta} d^2\boldsymbol{p} \Omega_{p_\alpha u_{s\beta}}(\mathbf{p}) = -\frac{A}{(2\pi)^2} \sum_{\eta=\pm1} \eta \int_{D_\eta} d^2\boldsymbol{p} \mathrm{Im} \frac{\langle \upsilon_{v\boldsymbol{p}} | \partial_{p_\alpha} H_{\boldsymbol{p}} | \upsilon_{c\boldsymbol{p}} \rangle \langle \upsilon_{c\boldsymbol{p}} | \partial_{u_{s\beta}} H_{\boldsymbol{p}} | \upsilon_{v\boldsymbol{p}} \rangle}{(\epsilon_{v\boldsymbol{p}} - \epsilon_{c\boldsymbol{p}})^2}. \tag{52}$$

Considering the atom with $l_s = 1$, $\alpha = x, \beta = x$, and transforming the derivative with respect to

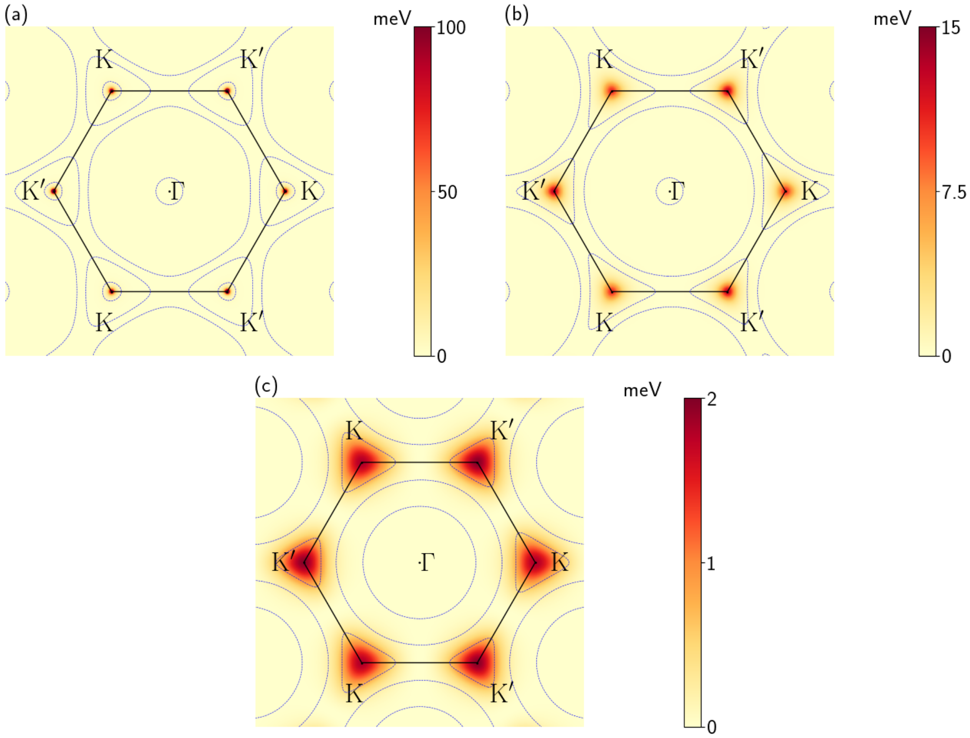


**Figure 7:** Same of Fig. 5, but for $\frac{\hbar^2}{\sqrt{M_s M_r}}\Omega_{u_{sx}u_{ry}}(\mathbf{k})$, with $l_s = 1$ and $l_r = -1$.

atomic position in a derivative with respect to the quasi momentum we obtain

$$Z^* = -\frac{A}{(2\pi)^2}\sum_{\eta=\pm1}\int_{D_\eta} d^2\boldsymbol{p}\,\mathrm{Im}\frac{\langle \upsilon_{v\boldsymbol{p}}|\,\partial_{p_x}H_{\boldsymbol{p}}\,|\upsilon_{c\boldsymbol{p}}\rangle\,\langle \upsilon_{c\boldsymbol{p}}|\,\partial_{u_{sx}}H_{\boldsymbol{p}}\,|\upsilon_{v\boldsymbol{p}}\rangle}{(\epsilon_{v\boldsymbol{p}}-\epsilon_{c\boldsymbol{p}})^2} \tag{53}$$

$$= -\frac{A}{(2\pi)^2}\sum_{\eta=\pm1}\eta\xi\int_{D_\eta} d^2\boldsymbol{p}\,\mathrm{Im}\frac{\langle \upsilon_{v\boldsymbol{p}}|\,\partial_{p_x}H_{\boldsymbol{p}}\,|\upsilon_{c\boldsymbol{p}}\rangle\,\langle \upsilon_{c\boldsymbol{p}}|\,\partial_{p_y}H_{\boldsymbol{p}}\,|\upsilon_{v\boldsymbol{p}}\rangle}{(\epsilon_{v\boldsymbol{p}}-\epsilon_{c\boldsymbol{p}})^2} \tag{54}$$

$$= \frac{A}{(2\pi)^2}\xi\sum_{\eta=\pm1}\eta\int_{D_\eta} d^2\boldsymbol{p}\,\Omega_{p_xp_y}(\boldsymbol{p}) = \frac{A}{2\pi}\xi\sum_{\eta=\pm1}(\eta)^1 C_\eta = \mathrm{sgn}(\Delta)\frac{A}{2\pi}\xi(1-|C|). \tag{55}$$

Notice that, as expected from symmetry considerations, we can obtain $Z^*$ also from the element

$\alpha = y, \beta = y$. In this case we would have

$$Z^* = -\frac{A}{(2\pi)^2}\sum_{\eta=\pm1}\int_{D_\eta} d^2\boldsymbol{p}\mathrm{Im}\frac{\langle\upsilon_{v\boldsymbol{p}}|\,\partial_{p_y}H_{\boldsymbol{p}}\,|\upsilon_{c\boldsymbol{p}}\rangle\,\langle\upsilon_{c\boldsymbol{p}}|\,\partial_{u_{sy}}H_{\boldsymbol{p}}\,|\upsilon_{v\boldsymbol{p}}\rangle}{(\epsilon_{v\boldsymbol{p}}-\epsilon_{c\boldsymbol{p}})^2} \tag{56}$$

$$= \frac{A}{(2\pi)^2}\sum_{\eta=\pm1}\eta\xi\int_{D_\eta} d^2\boldsymbol{p}\mathrm{Im}\frac{\langle\upsilon_{v\boldsymbol{p}}|\,\partial_{p_y}H_{\boldsymbol{p}}\,|\upsilon_{c\boldsymbol{p}}\rangle\,\langle\upsilon_{c\boldsymbol{p}}|\,\partial_{p_x}H_{\boldsymbol{p}}\,|\upsilon_{v\boldsymbol{p}}\rangle}{(\epsilon_{v\boldsymbol{p}}-\epsilon_{c\boldsymbol{p}})^2} \tag{57}$$

$$= -\frac{A}{(2\pi)^2}\sum_{\eta=\pm1}\eta\xi\int_{D_\eta} d^2\boldsymbol{p}\mathrm{Im}\frac{\langle\upsilon_{v\boldsymbol{p}}|\,\partial_{p_x}H_{\boldsymbol{p}}\,|\upsilon_{c\boldsymbol{p}}\rangle\,\langle\upsilon_{c\boldsymbol{p}}|\,\partial_{p_y}H_{\boldsymbol{p}}\,|\upsilon_{v\boldsymbol{p}}\rangle}{(\epsilon_{v\boldsymbol{p}}-\epsilon_{c\boldsymbol{p}})^2} \tag{58}$$

$$= \frac{A}{(2\pi)^2}\xi\sum_{\eta=\pm1}\eta\int_{D_\eta} d^2\boldsymbol{p}\Omega_{p_xp_y}(\boldsymbol{p}) = \frac{A}{2\pi}\xi\sum_{\eta=\pm1}(\eta)^1 C_\eta = \mathrm{sgn}(\Delta)\frac{A}{2\pi}\xi(1-|C|), \tag{59}$$

where it has been exploited that the Berry curvature is odd under the exchange of the order of the derivative $\Omega_{p_\beta p_\alpha}(\boldsymbol{p}) = -\Omega_{p_\alpha p_\beta}(\boldsymbol{p})$.
The molecular Berry curvature computation in the low energy limit follows an analogous procedure. We skip the general expression for $F_{s\alpha,r\beta}$ and specialise directly to $\mathcal{F}$, i.e. $r = s$ and $\alpha = x, \beta = y$—notice that the zone centre molecular Berry curvature vanishes if $\alpha = \beta$ because it reduces to the imaginary part of the integral of the modulus squared of a matrix element that has to be real; for the relations between the elements of $F_{s\alpha,r\beta}$ see Ref. [9]. We then write for the atom with $l_s = 1$

$$\mathcal{F} = \frac{\hbar^2}{M}\frac{A}{(2\pi)^2}\sum_n^{\mathrm{occ}}\int_{\mathrm{BZ}} d^2\boldsymbol{k}\Omega_{u_{sx}u_{sy}}(\mathbf{k}). \tag{60}$$

The low energy expression reads

$$\mathcal{F} = -\frac{\hbar^2}{M}\frac{A}{(2\pi)^2}\sum_{\eta=\pm1}\int_{D_\eta} d^2\boldsymbol{p}\mathrm{Im}\frac{\langle\upsilon_{v\boldsymbol{p}}|\,\partial_{u_{sx}}H_{\boldsymbol{p}}\,|\upsilon_{c\boldsymbol{p}}\rangle\,\langle\upsilon_{c\boldsymbol{p}}|\,\partial_{u_{sy}}H_{\boldsymbol{p}}\,|\upsilon_{v\boldsymbol{p}}\rangle}{(\epsilon_{v\boldsymbol{p}}-\epsilon_{c\boldsymbol{p}})^2} \tag{61}$$

$$= \frac{\hbar^2}{M}\frac{A}{(2\pi)^2}\sum_{\eta=\pm1}(\eta)^2\xi^2\int_{D_\eta} d^2\boldsymbol{p}\mathrm{Im}\frac{\langle\upsilon_{v\boldsymbol{p}}|\,\partial_{p_y}H_{\boldsymbol{p}}\,|\upsilon_{c\boldsymbol{p}}\rangle\,\langle\upsilon_{c\boldsymbol{p}}|\,\partial_{p_x}H_{\boldsymbol{p}}\,|\upsilon_{v\boldsymbol{p}}\rangle}{(\epsilon_{v\boldsymbol{p}}-\epsilon_{c\boldsymbol{p}})^2} \tag{62}$$

$$= -\frac{\hbar^2}{M}\frac{A}{2\pi}(\xi)^2\sum_{\eta=\pm1}\eta^2\int_{D_\eta} d^2\boldsymbol{p}\Omega_{p_\beta p_\alpha}(\boldsymbol{p}) = -\frac{\hbar^2}{M}\frac{A}{2\pi}(\xi)^2\sum_{\eta=\pm1}\eta^2 C_\eta = -\frac{\hbar^2}{M}\frac{A}{2\pi}(\xi)^2 C. \tag{63}$$

# 5 Valley Chern number in the Kane-Mele model

Since the Kane-mele model is symmetric under time reversal, the Chern number is vanishing for any choice of the parameters and so the sum of the Chern numbers computed in a neighbourhood of the two valleys has to vanish. Nevertheless, as plotted in Figure 8, the two valleys Chern number are vanishing in the topologically non trivial phase, whereas they are equal and opposite in the trivial one. The topological nature of the system is described by the $\mathcal{Z}_2$ topological index, that is calculated here exploiting the flow of the hybrid Wannier centroids [10]–[12]. The valley Chern number in this model is related to the topological index by the relation $C_v = 1 - \mathcal{Z}_2$ so that the Born Effective charges, measuring the valley Chern number of the system, provide also a direct quantification of the topological index of the system.

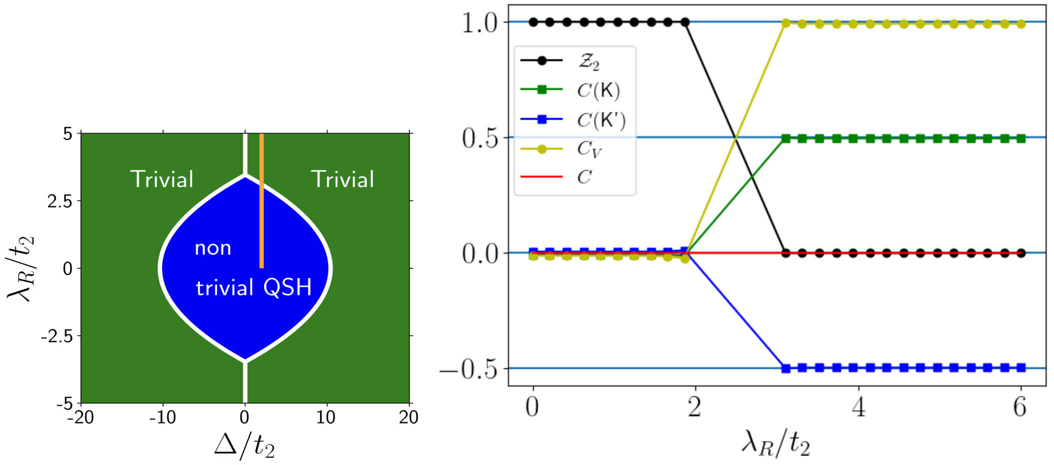


**Figure 8:** (Left) Numerical topological phase diagram of the Kane-Mele model in the $(\Delta/t_2, \lambda_R/t_2)$ plane for $t_2 = 0.02$ eV. The plot on the right is performed along the vertical orange line ($\Delta = 0.1$ eV). (Right) Chern number, Chern number restricted around each of the two valleys, valley Chern number and $\mathcal{Z}_2$ topological index in the Kane-Mele model as a function of the Rashba coupling strength $\lambda_R$

# 6 Stability of the results

The tight-binding description of the electronic bands of graphene is significantly improved by the inclusion of higher order neighbours in the model up to the fifth ones [6]. In order to prove the stability of the results with respect to changes in the band structure that does not spoil the behaviour in the two valleys, the Kane-Mele model is enriched by neighbours up to the fifth with the parameters presented in [6]. As shown in Fig. 9, also in this case the Born effective charges undergo the same transition described in the main text. This confirms the hypothesis that the results mostly depend on the band dispersion located around in the two valleys. Notice that the electron-phonon coupling is always kept up to the nearest-neighbours level, by virtue of the fact that the second nearest neighbour coupling is vanishing at the $\Gamma$. In fact, second nearest neighbours are ions of the same species, in different cells, that for zone center phonons perform the same oscillation. Therefore, there is no relative displacement. Thus, only a neighbours connecting ions of different species can give rise to a non zero electron-phonon term. The model may include a non vanishing third order nearest neighbours electron-phonon coupling but the strength of the coupling is expected to be much smaller with respect to the dominant contribution.

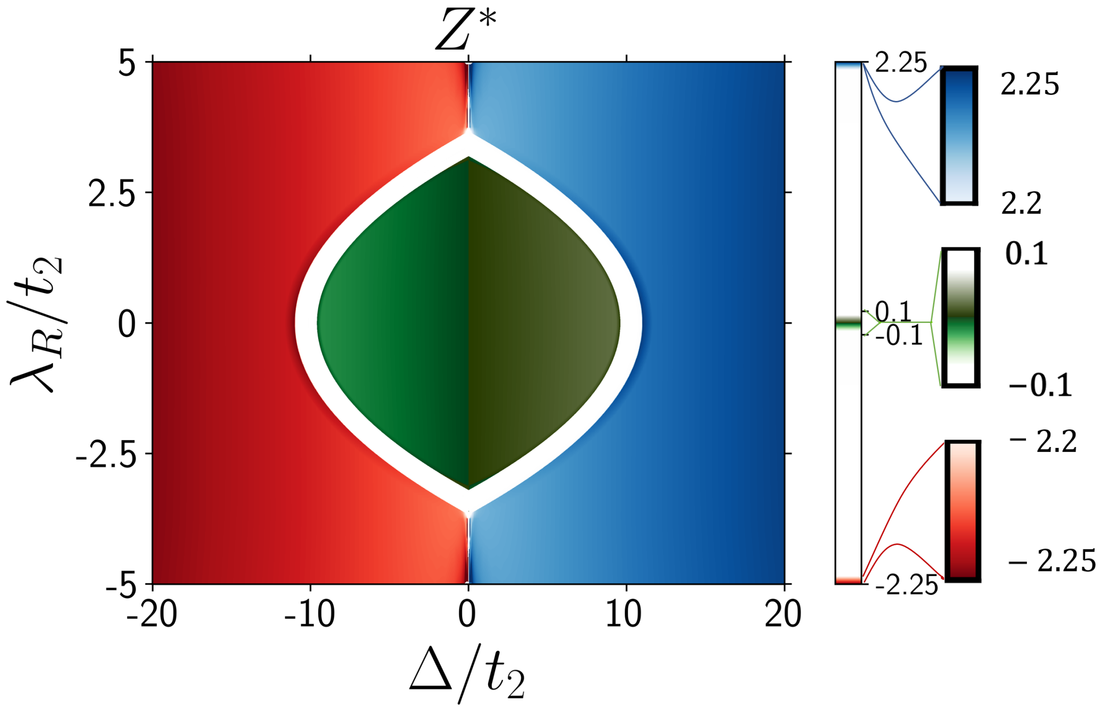


**Figure 9:** Same analysis as in the main text, performed for the Kane-Mele model including up to fifth nearest neighbours.

## References


[1] O. Bistoni, P. Barone, E. Cappelluti, L. Benfatto, and F. Mauri, "Giant effective charges and piezoelectricity in gapped graphene," *2D Materials*, vol. 6, no. 4, p. 045 015, 2019. DOI: 10.1088/2053-1583/ab2ce0.

[2] F. Macheda, P. Barone, and F. Mauri, "Electron-phonon interaction and longitudinal-transverse phonon splitting in doped semiconductors," *Phys. Rev. Lett.*, vol. 129, p. 185 902, 18 2022. DOI: 10.1103/PhysRevLett.129.185902.

[3] F. Macheda, T. Sohier, P. Barone, and F. Mauri, "Electron-phonon interaction and phonon frequencies in two-dimensional doped semiconductors," *Phys. Rev. B*, vol. 107, p. 094 308, 9 2023. DOI: 10.1103/PhysRevB.107.094308.

[4] R. Winkler, *Spin—Orbit Coupling Effects in Two-Dimensional Electron and Hole System*. Springer Berlin, Heidelberg, 2003.

[5] P.-O. Löwdin, "Partitioning technique, perturbation theory, and rational approximations," *International Journal of Quantum Chemistry*, vol. 21, no. 1, pp. 69–92, 1982. DOI: https://doi.org/10.1002/qua.560210105. eprint: https://onlinelibrary.wiley.com/doi/pdf/10.1002/qua.560210105.

[6] P. Venezuela, M. Lazzeri, and F. Mauri, "Theory of double-resonant raman spectra in graphene: Intensity and line shape of defect-induced and two-phonon bands," *Phys. Rev. B*, vol. 84, p. 035 433, 3 2011. DOI: 10.1103/PhysRevB.84.035433.

[7] F. D. M. Haldane, "Model for a quantum hall effect without landau levels: Condensed-matter realization of the "parity anomaly"," *Phys. Rev. Lett.*, vol. 61, pp. 2015–2018, 18 1988. DOI: 10.1103/PhysRevLett.61.2015.

[8] L. Graziotto, F. Macheda, T. Sohier, M. Calandra, and F. Mauri, "Theory of infrared double-resonance raman spectrum in graphene: The role of the zone-boundary electron-phonon enhancement," *Phys. Rev. B*, vol. 109, p. 075 420, 7 2024. DOI: 10.1103/PhysRevB.109.075420.

[9] D. Saparov, B. Xiong, Y. Ren, and Q. Niu, "Lattice dynamics with molecular berry curvature: Chiral optical phonons," *Phys. Rev. B*, vol. 105, p. 064 303, 6 2022. DOI: 10.1103/PhysRevB.105.064303.

[10] A. A. Soluyanov and D. Vanderbilt, "Computing topological invariants without inversion symmetry," *Phys. Rev. B*, vol. 83, p. 235 401, 23 2011. DOI: 10.1103/PhysRevB.83.235401.

[11] M. Taherinejad, K. F. Garrity, and D. Vanderbilt, "Wannier center sheets in topological insulators," *Phys. Rev. B*, vol. 89, p. 115 102, 11 2014. DOI: 10.1103/PhysRevB.89.115102.

[12] D. Vanderbilt, *Berry Phases in Electronic Structure Theory*. Cambridge University Press, 2018.
